# Supplementary material for: RAId_aPS: MS/MS analysis with multiple scoring functions and spectrum-specific statistics
Source: arXiv:0806.2685 ancillary file (2010-09-16)
Supplement: Supplementary file 1 [file RAId_aPs_support.pdf]

# Supporting Materials for RAId_aPS: MS/MS analysis with multiple scoring functions and spectrum-specific statistics

Gelio Alves[1], Aleksey Y. Ogurtsov[1] and Yi-Kuo Yu[1,*]

**1 National Center for Biotechnology Information, National Library of Medicine, National Institutes of Health, Bethesda, MD 20894**

∗ **E-mail:yyu@ncbi.nlm.nih.gov**

## Text S1: Spectral Filtering and Scoring Functions

The main objective of this appendix is to document what we found from the source codes of various search methods about their spectral filtering strategies. Although effort is invested to faithfully reproduce these filtering strategies, we do no intend to provide a logical explanation of these filtering methods. Readers interested in obtaining logical explanations of these strategies should contact the original code authors. There also exist other heuristics in various scoring functions that we chose to ignore. As shown in Figure 6 and Figure S6 of the supporting information, and in dashed curves of Figures S8 and S9, the performance of these scoring functions without heuristics do not suffer from poorer retrieval compared to their original implementations with heuristics included.

### Notation

Before we begin documentation of the filtering strategies associated with different scoring functions as well as our implementation of these scoring functions, we define a set of notations.

- `mw` precursor ion molecular weight at charge +1 state
- $z$ peptide/fragment charge state
- $m/z$ mass over charge
- $m_i$ molecular mass of fragment $i$ in the MS/MS spectrum
- $\Delta m_i$ mass disagreement between the theoretical mass of fragment $i$ and $m_i$.
- $I_i$ peak intensity of an observed $m_i$
- `hw` highest observed molecular weight
- `lw` lowest observed molecular weight
- $\pi$ a peptide sequence
- $\delta m$ MS/MS spectrum $m/z$ accuracy
- Da Dalton
- $T(\pi)$ represents the set of theoretical peaks used for scoring or the total number of items in that set.
- $l(\pi)$ length of peptide $\pi$, the total number of amino acids in peptide $\pi$.
- $H$ molecular weight of a hydrogen atom

## RAId Score Filtering and Scoring Function

1) The details of RAId score filtering are explained in RAId_DbS original publication [1].

2) The RAId scoring function (also used in RAId_DbS) is define as

$$\text{RAId } S(\pi) = \frac{1}{T(\pi)} \sum_{i=1}^{T(\pi)} \ln(I_i)\; e^{-\Delta m_i} \theta(1 - \Delta m_i),$$

with the default theoretical peaks for scoring $T(\pi) = \{b_n, y_n\}_{n=1}^{l(\pi)-1}$ and with $l(\pi)$ representing the number of amino acids in peptide $\pi$.

## X!Tandem Filtering and Hyperscore

1) $m/z$ fragments that are within $\pm 0.95$ Da of each other are removed from the MS/MS spectrum. When two fragments are within $\pm 0.95$ Da of each other the fragment with the highest intensity is kept.

```
for(i = lw; i < hw; i = i+1)
   for(j = lw+1; j ≤ hw; j = j+1)
     do
     if ((m_i - m_j) < 0.95   &&   I_i < I_j )  m_i = 0 ;   I_i = 0 ;
```

2) $m/z$ fragments that are in the mass range $(x - 5/z, x + 5/z)$ are removed from the MS/MS spectrum, where $x = 1.00727 + (\mathtt{mw} - 1.00727)/z$.

3) $m/z$ fragments that are lighter than 150 Da are removed from the MS/MS spectrum.

4) The filtered spectrum is normalized to have maximum intensity 100 and fragments with normalized intensity less than 1 are removed from the spectrum.

5) Try to determine if the spectrum is purely noise.

```
if(z=1 || z=2)  x = mw - 600
else   x = mw/z
if( Heaviest Filtered Fragment  < x)
   exit  (spectrum is noisy)
else if( Total Number of Filtered Fragments < 5)
   exit  (spectrum is noisy)
```

6) m/z fragments that are within $\pm 1.5$ Da are removed from the spectrum. When two fragments are within $\pm 1.5$ Da of each other the fragment with the highest intensity is kept, as shown in step 1).

7) The final filtered spectrum consists at most 50 fragments having the highest intensities.

8) The molecular weights of the fragments in the filtered spectrum are transformed to integer values using the MS/MS spectrum mass accuracy ($\delta m$).

$m_i = \mathtt{int}[\frac{m_i}{\delta m} + 0.5]$

9) After the transformation above, the mass indices to either sides of $m_i$ are initialized as follows:

```
for(i=1; i < int [mw /δm]; i = i+1)
    do
    if( I_{i-1} < I_i) I_{i-1} = I_i
    if( I_{i+1} < I_i) I_{i+i} = I_i
```

*Note: To speed up the code in RAId_aPS implementation the intensity is further scale by multiplying it by a factor of 0.1: $I_i = 0.1 \times I_i$.

10) Theoretical fragments chosen for scoring $T(\pi) = \{b_n, y_n\}_{n=1}^{l(\pi)-1}$. For a precursor ion with charge $z = 2$, the score is give by:

$$\text{Hyperscore } S(\pi) = 4 \log_{10} \left[ 10 \left( \sum_{i=1}^{T(\pi)} I_i \right) b!\, y! \right]$$

The multiplication factor of "10" in the above scoring function is introduced because RAId_aPS scaled the intensity by a factor of 0.1 as mentioned above. To keep RAId_aPS's run time reasonable, for parent ion in higher charge state, RAId_aPS scoring deviates from the X!Tandem Hyperscore. Basically, counter $b(y)$ totals the number of $b$-($y$-)type of evidence peaks without separating them further into different charge states.

## Crux Filtering and XCorr

1) The intensities present in the MS/MS spectrum are transformed by taking the square root of the original intensities.

$$I_i = \sqrt{I_i}$$

2) $m/z$ fragments that are in the mass range $(x - 15, x + 15)$ are removed from the MS/MS spectrum, where $x = (\texttt{mw} + z - 1.0)/z$.

3) $m/z$ fragments that are greater than $x$ are removed from the MS/MS spectrum, where $x = (\texttt{mw} + z - 1 + 50)$.

4) Observed $m/z$ fragments in the MS/MS spectrum are transformed to integer values using a mass grid where neighboring points are spaced by 1.0005079 Da.

```
x = (mw + z - 1 + 50)
for(i = 0; i ≤ x; i = i+1) s[i]=0
for(i = 0; i ≤ x; i = i+1)
    do
    m_i = int[m_i/1.0005079 + 0.5]
    if(s[m_i]< I_i) s[m_i] = I_i
```

5) The MS/MS spectrum's m/z range is divided into 10 mass regions. The width of each region is equal to the heaviest observed fragment molecular weight `hw` divided by 10.
$mr = \texttt{int}[\texttt{hw}/10]$
The 10 regions are: $[0, mr), [mr, 2mr), [2mr, 3mr), \ldots,$ and $[9mr, 10mr)$

6) The peak intensities within each region, if m/z fragments exist, are normalized to have

maximum intensity 50. If no mass fragment is present in a given region, the maximum region intensity is set to 0.

7) The final filtered spectrum is obtained by applying the following operation to the spectrum intensities

```
x = (mw + z - 1 + 50)
for( i = 0; i < x; i = i+1
   do  for(v = 0, j = i-75; j ≤ i+75; j++)
         do  if(j ≥0 &&  j < x)  v = v + s[j]
   I_i = s[i] - v/150
```

8) The XCorr score is computed by taking the dot product between the theoretical fragments $T(\pi)$ and the filtered spectrum $I_i$. The default series used for scoring is $T(\pi) = \{b_n, y_n, b_n-H, b_n+H, y_n-H, y_n+H, b_n-H_2O, b_n-NH_3, y_n-NH_3, a_n\}_{n=1}^{l(\pi)-1}$, with each series contributing to the score respectively weighted by $w_i = \{50, 50, 25, 25, 25, 25, 10, 10, 10, 10\}$.

$$\text{XCorr } S(\pi) = \frac{1}{10000} \sum_{i=1}^{T(\pi)} w_i I_i \ .$$

Note: To speed up the code, RAId_aPS implements XCorr with different scales for intensity and weight factors. First, the peak intensity is scale down by a factor of ten: $I_i = 0.1 \times I_i$.

Second, the weight factors are scaled down by a factor of 50,
thus $w_i = \{1, 1, 0.5, 0.5, 0.5, 0.5, 0.2, 0.2, 0.2, 0.2\}$. Since we are absorbing a factor 1/50 into the weights and another factor 1/10 into the peak intensities, the Xcorr score in RAId_aPS reads

$$\text{XCorr } S(\pi) = \frac{1}{20} \sum_{i=1}^{T(\pi)} w_i I_i \ ,$$

because the factor 1/10000 can be written as

$$\frac{1}{10000} = \frac{1}{50} \times \frac{1}{10} \times \frac{1}{20} \ .$$

## K-score Filtering and Scoring Function

1) The intensities present in the MS/MS spectrum are transformed by taking the square root of the original intensities.

$$I_i = \sqrt{I_i}$$

2) $m/z$ fragments less than $x$ are removed from the MS/MS spectrum, where $x = (\texttt{mw} + (z - 1) * 1.00075) \times 2/z + 10.5$.

3) The observed $m/z$ fragments in the MS/MS spectrum are transformed to integer values using a mass grid where neighboring points are spaced by 1.0005 Da.

```
for(i = 0; i ≤ (mw+128); i = i+1) s[i]=0
for(i = 0; i ≤ hw; i = i+1)
   do
   m_i = int [m_i/1.0005 + 0.5]
```

```
if (s[m_i]< I_i)  s[m_i] = I_i
```

4) The spectrum's m/z range is partitioned into intervals with the number of intervals depending on the value of $R$, see below.

```
x = (mw + (z-1)*1.00075)× 2/z + 10.5
R = min(x,hw+10)-lw
```

The number of partitions N($R$) is determined by the condition below

$$\mathrm{N}(R) = \begin{cases} 10 & : \quad R > 3000 \\ 9 & : \quad R > 2500 \\ 8 & : \quad R > 2000 \\ 7 & : \quad R > 1500 \\ 6 & : \quad R > 1000 \\ 5 & : \quad R > 0 \end{cases}$$

5) Within each partition the spectrum is scaled such that the maximum peak intensity in each interval equals to the maximum intensity in the MS/MS spectrum right after step 1). Peaks with intensities that are less than 5 percent of the maximum spectrum intensity are removed.

6) The spectrum is normalized to a unit vector.

```
for(x = 0, i = 0; i ≤ hw; i = i+1) x = x+s[i]× s[i]
for(i = 0; i ≤ hw; i = i+1) s[i] = s[i]/√x
```

7) The final filtered spectrum is obtained by applying the following transformation to the peak intensities

```
for(i = 0; i ≤ hw; i = i+1)
   do  for(v = 0, j = i-50; j ≤ i+50; j++)
          do  if(j ≥ 0  &&  j ≤ hw)  v = v+s[j]
   if (s[i]- v/101 > 0 )
          I_i = s[i] - v/101
```

8) The K-score is computed by taking the dot product between the theoretical fragments $T(\pi)$ and the filtered spectrum $I_i$. The default fragmentation series used for scoring are $T(\pi) = \{b_n, y_n, b_n - H, b_n + H, y_n - H, y_n + H\}_{n=1}^{l(\pi)-1}$, with each series contributing to the score respectively weighted by $w_i = \{1, 1, 0.5, 0.5, 0.5, 0.5\}$.

$$\text{K–Score} \quad S(\pi) = \frac{1000\ \ln(l)}{3\sqrt{l}} \sum_{i=1}^{T(\pi)} w_i I_i$$

# Supporting Figures

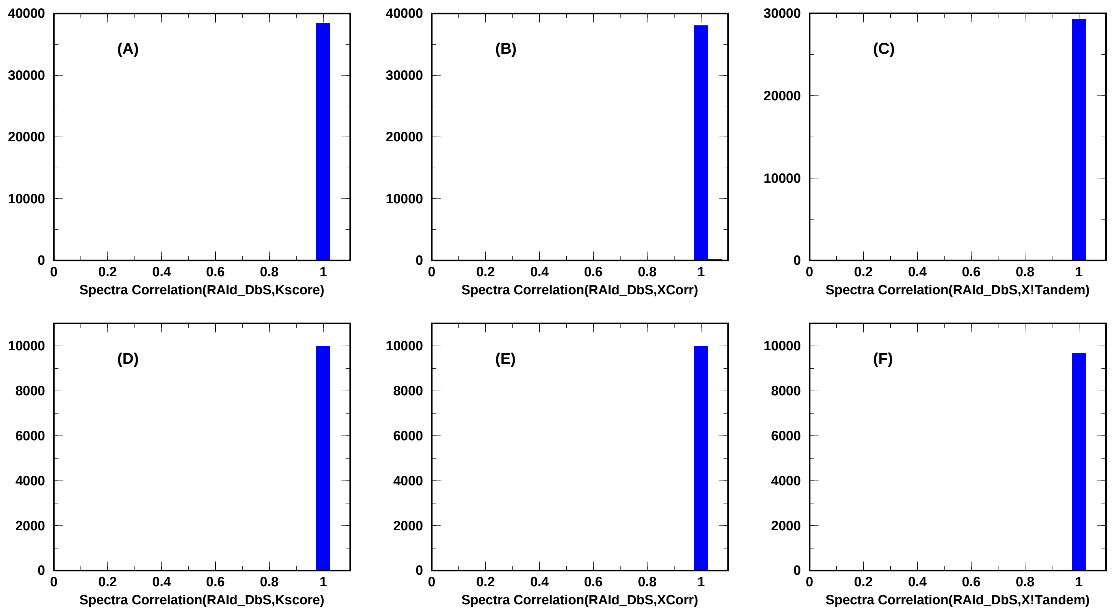


**Figure S1.** Filtering accuracy assessment. For every raw spectrum, one generates six filtered spectra: three associated with Hyperscore/XCorr/K-score implemented in RAId_aPS and the other three respectively produced by X!Tandem/Crux/X!Tandem(with K-score plug-in). The mass fragments of every filtered spectrum are then read to a mass grid. The spectrum is then viewed as a vector with non-vanishing components only at the component/mass indices populated. One then normalizes each *filtered* spectrum vector into unit length. An inner product of any two filtered spectral vectors represents the correlation between them. When the spectral quality does not pass a method-dependent threshold, the corresponding filtering protocol may turn the raw spectrum into a null spectrum without further searching the database. Therefore the total number of spectra passing through the filtering stage might be smaller than the total number of raw spectra, which is also reflected in the histograms. Two sets of data are used for this evaluation. The centroid data, consisting of 38,424 spectra, are from the ISB data set [2]. The profile data, consisting of 10,000 spectra, are from the NHLBI data set [3]. Panel A(D) shows the histogram of correlation between the RAId_aPS K-score and the X!Tandem K-score plug-in using centroid(profile) data. Panel B(E) shows the histogram of correlation between the RAId_aPS XCorr and the Crux XCorr using centroid(profile) data. Panel C(F) shows the histogram of correlation between the RAId_aPS Hyperscore and the X!Tandem Hyperscore using centroid(profile) data. The correlation strength being always one means that RAId_aPS is able to faithfully reproduce the filtering strategies originally designed for Hyperscore, XCorr, and K-score.

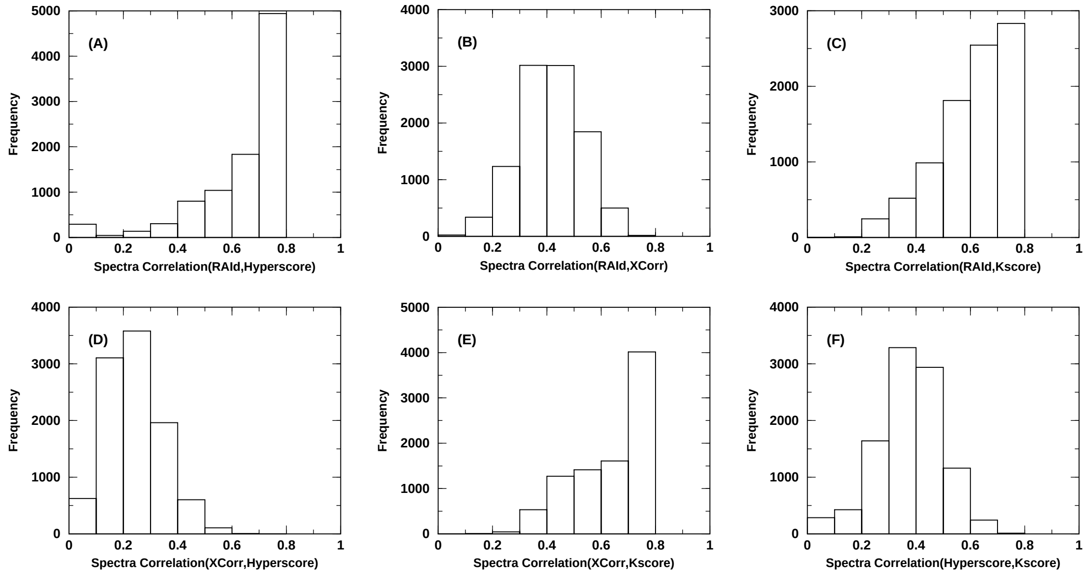


**Figure S2.** Histograms of correlations between filtering strategies. This Figure is the same as Figure 3 except that the 10, 000 raw spectra used are profile data from the NHLBI data set. [3]

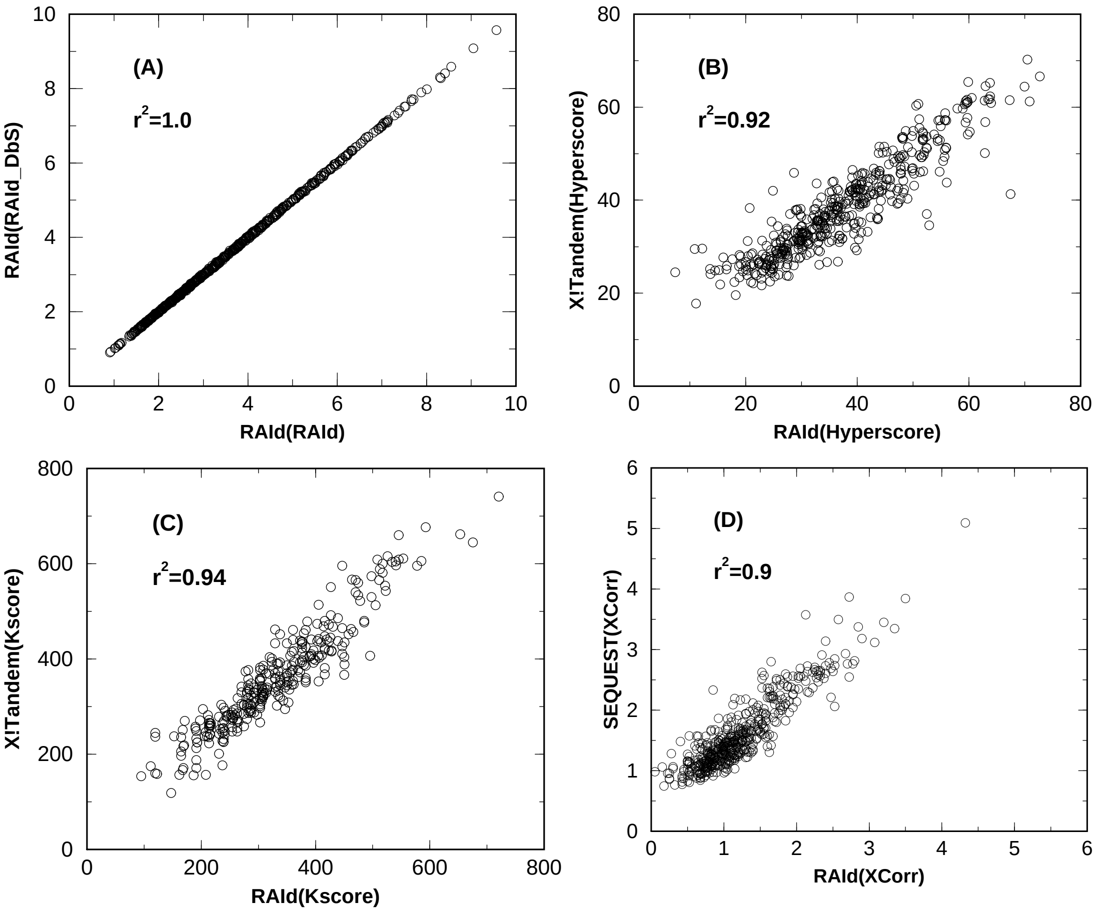


**Figure S3.** Score correlations. A subset of the NHLBI profile data set [3] was used to perform this evaluation. For each scoring function, when the best hit per spectrum (analyzed using the analysis program that the scoring function was originally used for) is a true positive, that candidate peptide is scored again using the corresponding scoring function implemented in RAId_aPS. Each true positive best hit thus gives rise to two scores and plotted using the following rule: the first score is used as the ordinate while the second score (from RAId_aPS) is used as the abscissa. Including 500 spectra, panel A is for the RAId score. Panel B is for Hyperscore and contains 495 spectra. The result of K-score is shown in panel C with 310 spectra. Shown with 500 spectra, panel D documents the results for XCorr.

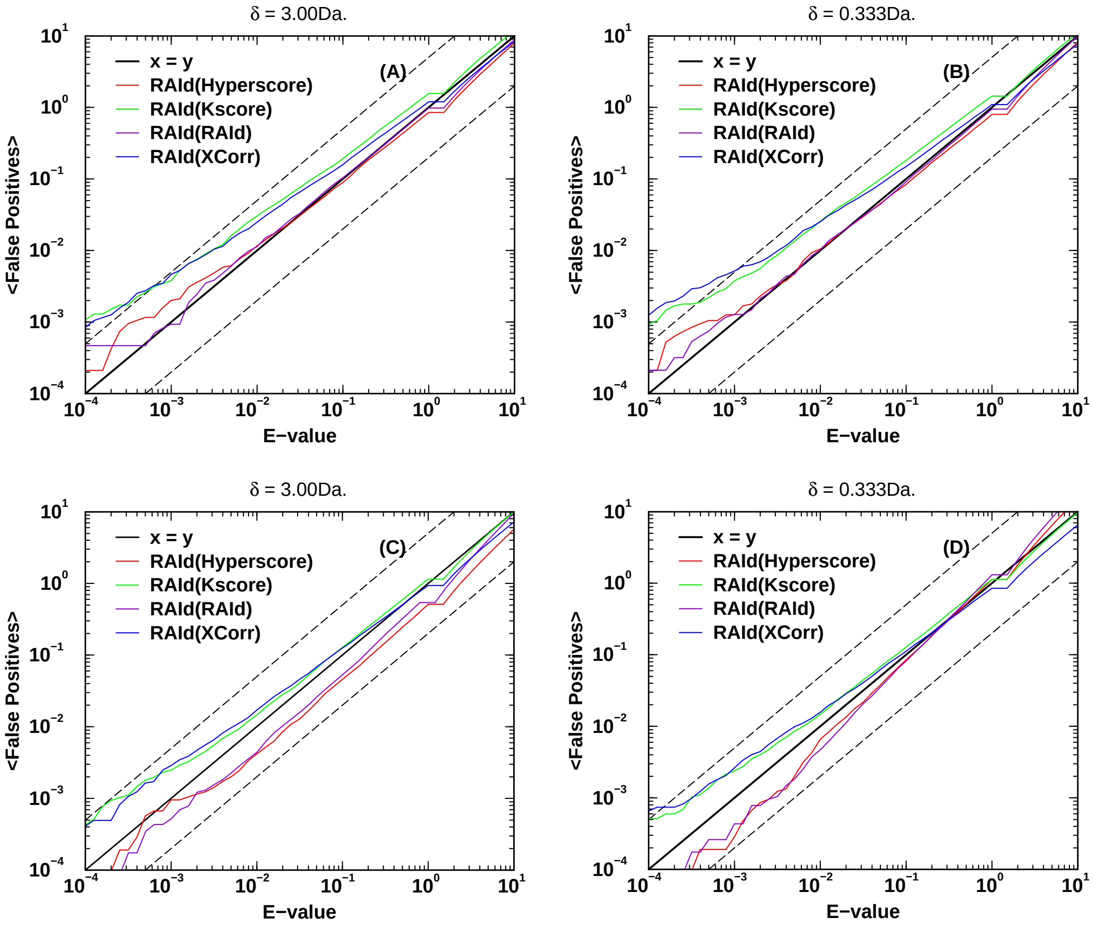


**Figure S4.** E-value accuracy assessment. The agreement between the reported $E$-value and the textbook definition is examined using profile data (panel (A-B), $10,000$ spectra of the NHLBI data set) as well as centroid data (panel (C-D), A1-A4 subsets of ISB data set). The NCBI's nr (of size 500 MB) database with true positives removed is used for this assessment. The molecular weight range considered while searching the database is $[MW - \delta, MW + \delta]$. In each panel, the dashed lines, corresponding to $x = 5y$ and $x = y/5$, are used to provide a visual guide regarding how close/off the experimental curves are from the theoretical curve.

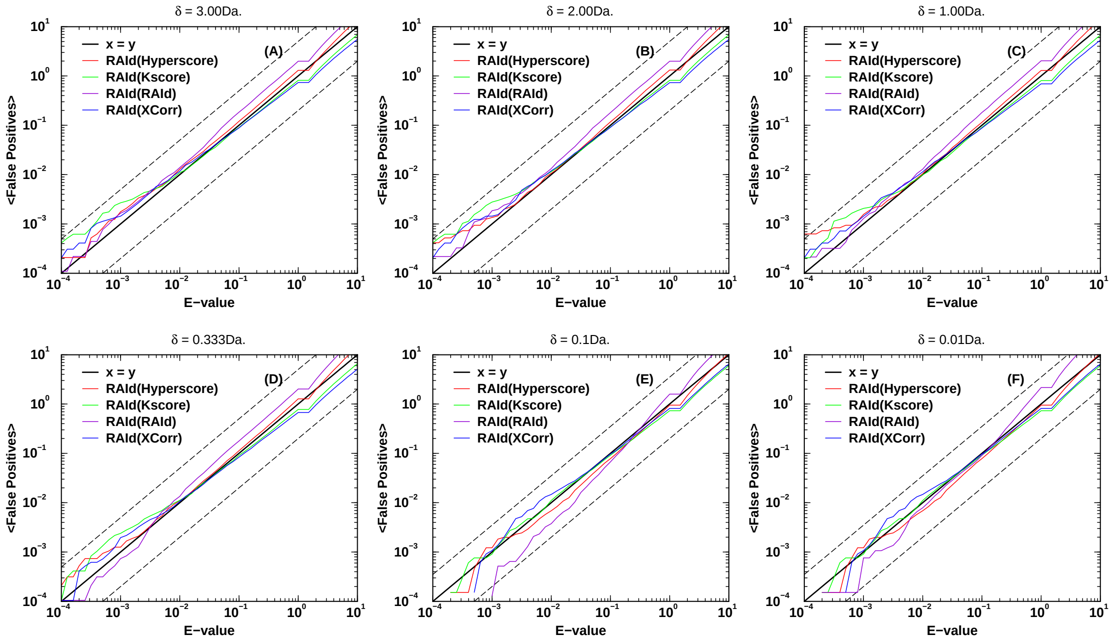


**Figure S5.** E-value accuracy assessment. The agreement between the reported $E$-value and the textbook definition is examined using profile data (the NHLBI data set: $10,000$ spectra). The random database size used is 500 MB. The molecular weight range considered while searching the database is $[MW - \delta, MW + \delta]$. In each panel, the dashed lines, corresponding to $x = 5y$ and $x = y/5$, are used to provide a visual guide regarding how close/off the experimental curves are from the theoretical curve.

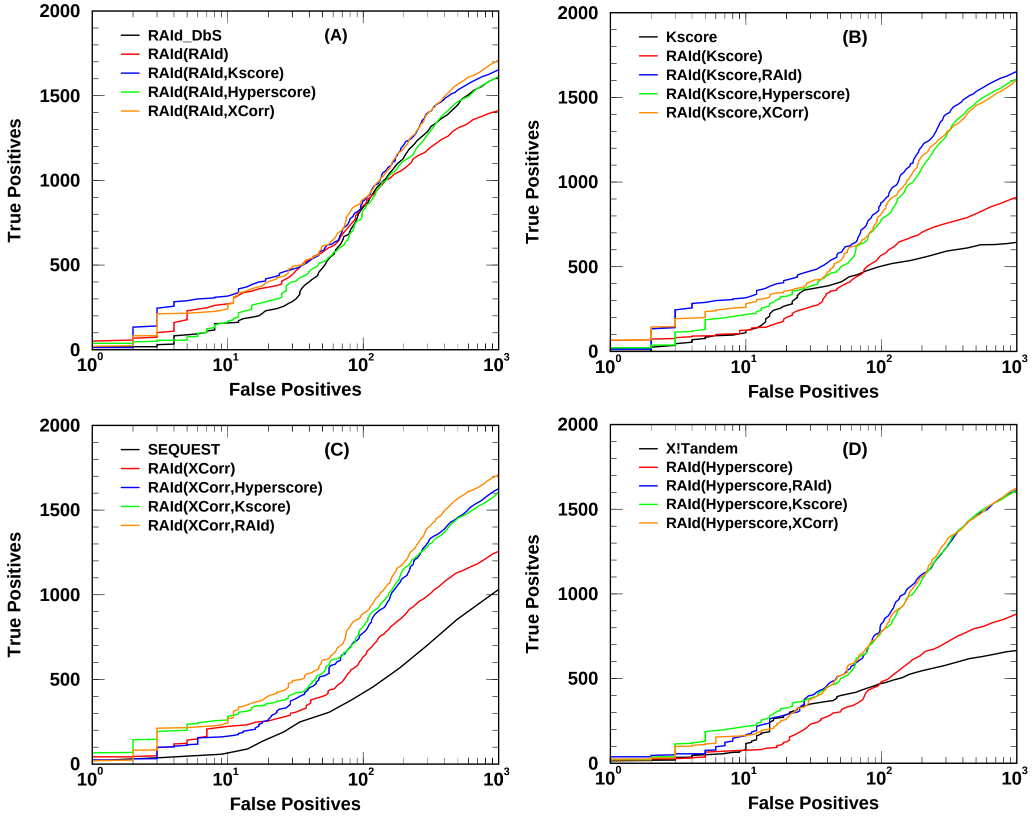


**Figure S6.** ROC curves for the profile data (NHLBI data set [3]). For each of the four scoring functions considered, a set of ROC curves is shown. These ROC curves include the results from running the designated program associated with that scoring function, the results from running RAId_aPS in the database search mode, and the results from combining with each one of the three other scoring functions. Panel (A) shows the results from RAId score, whose designated program is RAId_DbS. Panel (B) displays the results from K-score, whose designated program is X!Tandem. Panel (C) exhibits the results from XCorr, which is mostly employed by SEQUEST. Panel (D) presents the results from Hyperscore, whose designated program is also X!Tandem.

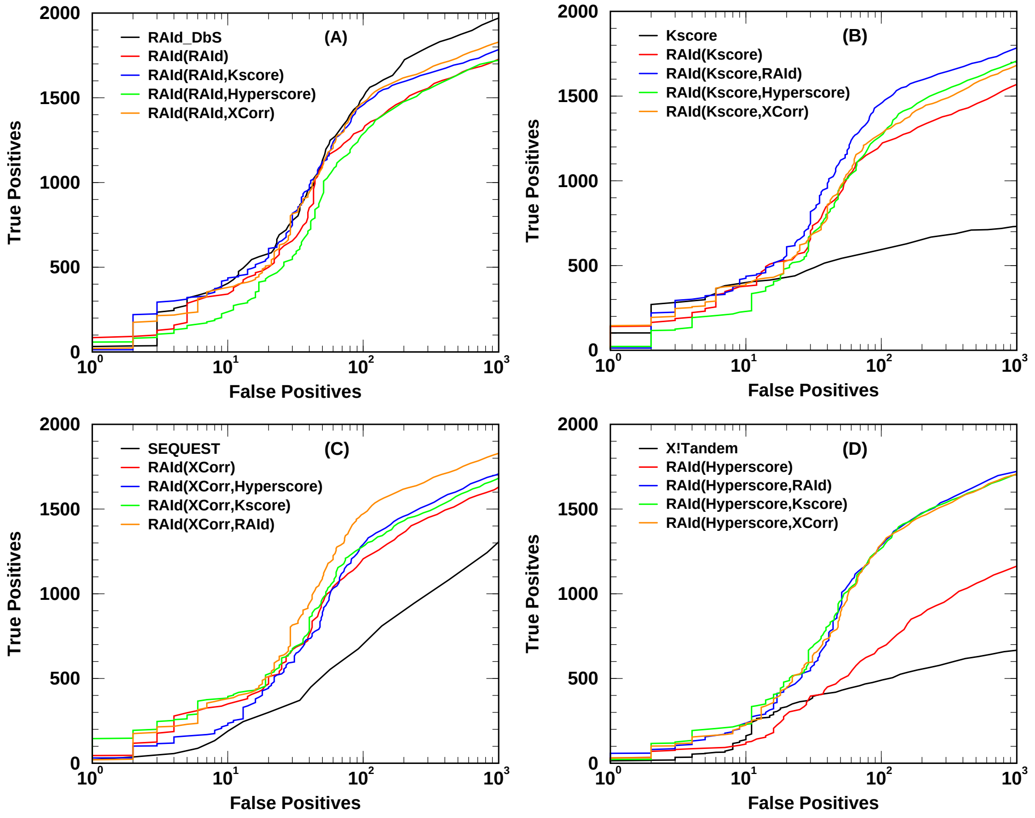


**Figure S7.** ROC curves for the profile data (NHLBI data set [3]) when considering only the best hit per spectrum. For each of the four scoring functions considered, a set of ROC curves is shown. These ROC curves include in the consideration only the best hit per spectrum from running the designated program associated with that scoring function, the best hit per spectrum from running RAId_aPS in the database search mode, and the best hit per spectrum from combining with each of the three other scoring functions. Panel (A) shows the results from RAId score, whose designated program is RAId_DbS. Panel (B) displays the results from K-score, whose designated program is X!Tandem. Panel (C) exhibits the results from XCorr, which is mostly employed by SEQUEST. Panel (D) presents the results from Hyperscore, whose designated program is also X!Tandem.

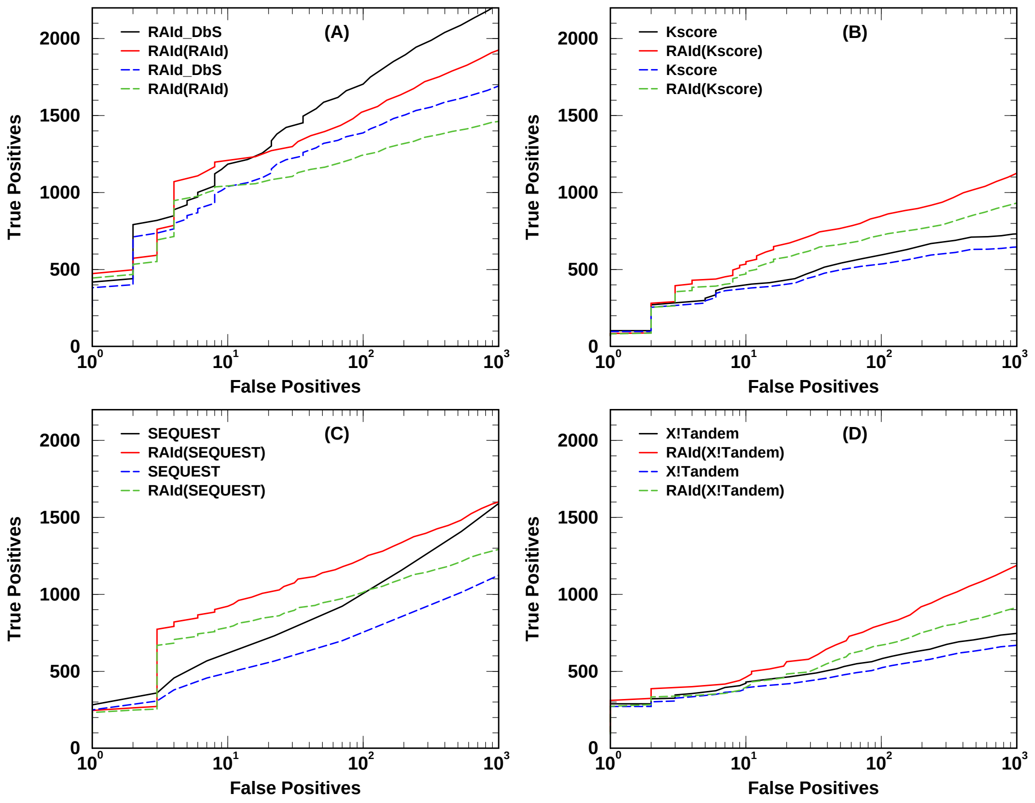


**Figure S8.** ROC curves when highly homologous proteins [1] are also counted as true positive proteins. Plots done this way are analogous to the ROC plots obtained using a decoy database to estimate the number of false positives. Each panel displays the results of a scoring function. The resulting ROC curves from using RAId_aPS implementation and the implementation in the original search program are both shown. The results from profile data (NHLBI data set [3]) are shown in solid curves, while the results from centroid data (A1-A4 of ISB data set [2]) are shown in long-dash curves. Panels (A,B,C,D) respectively display the results from using RAId score, K-score, XCorr, and Hyperscore. Except for RAId score, the RAId_aPS implemented scoring functions performs comparably to the original implementation in other search methods.

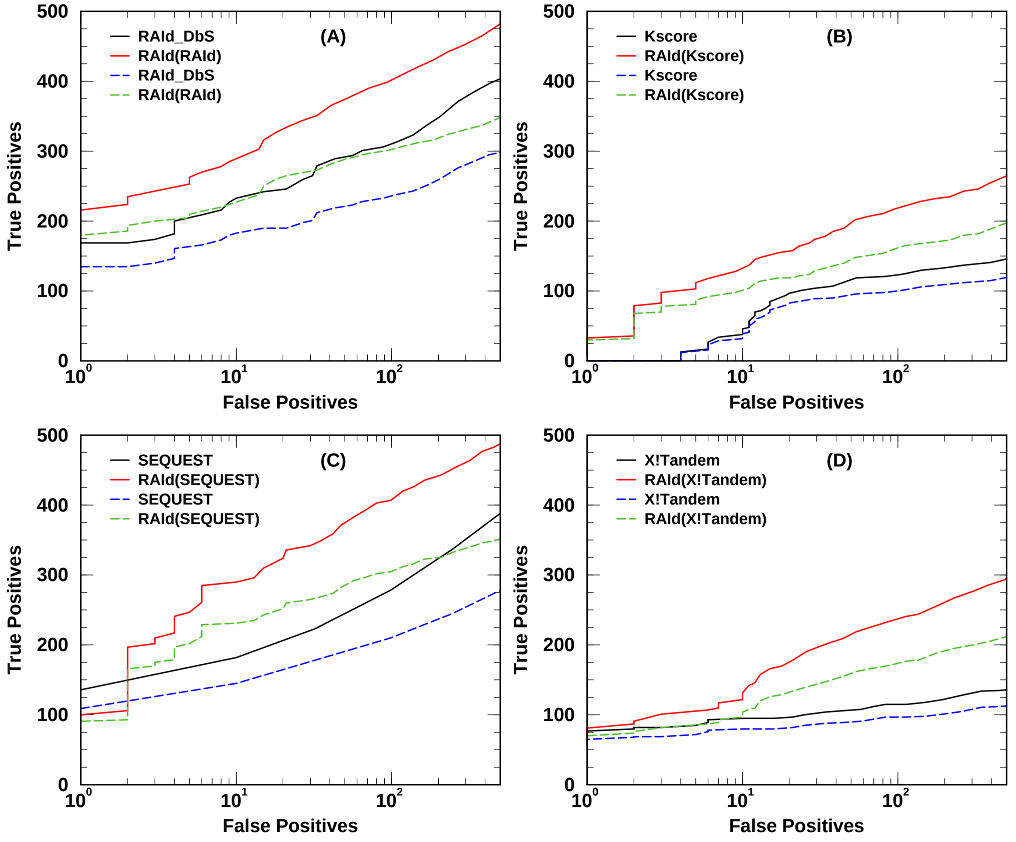


**Figure S9.** ROC curves when highly homologous proteins [1] are removed from the nr database and thus are not counted towards true positives or false positives. Each panel displays the results of a scoring function. The resulting ROC curves from using RAId_aPS implementation and the original implementation in other search program are both shown. The results from profile data (NHLBI data set [3]) are shown in solid curves, while the results from centroid data (A1-A4 of ISB data set [2]) are shown in long-dash curves. Panels (A,B,C,D) respectively display the results from using RAId score, K-score, XCorr, and Hyperscore. The RAId_aPS implemented scoring functions performs comparably to the original implementation in other search methods.

## References

1. Alves G, Ogurtsov AY, Yu YK (2007) RAId_DbS: Peptide identification using database searches with realistic statistics. Biology Direct 2: 25.

2. Keller A, Samuel P, Nesvizhskii AI, Stolyar S, Goodlett DR, et al. (2002) Experimental protein mixture for validating tandem mass spectral analysis. OMICS 6: 207-212.

3. Alves G, Ogurtsov AY, Wu WW, Wang G, Shen RF, et al. (2007) Calibrating E-values for $MS^2$ library search methods. Biology Direct 2: 26.
